# Supplementary material for: CAT: A GPU-Accelerated FHE Framework with Its Application to High-Precision Private Dataset Query
Source: arXiv:2503.22227 source file (2025-03-28)
Supplement: Supplementary file 1 [file sec8-appendix.tex]

%\subsection*{Appendix A: Algorithm for calculating modulus}
%\textbf{Appendix A: Algorithm for calculating modulus}
\begin{algorithm}[!ht]
\caption{Whole procedure for calculating of modulus for two big integers on GPU using method in \cite{will2014computing}}
\label{module_gpu}
\begin{algorithmic}[1]
\Procedure{Set\_higher\_bits\_0(T)}{}
    \State $\text{ploy\_mod\_Y} \gets (2^{len_Y} \mod \text{Y})$
    \While{$(\text{T} \ge (\text{1} \ll len_Y)) $}
        \State $\text{T} \gets \text{T} - (\text{1} \ll len_Y)  + \text{ploy\_mod\_Y} $
    \EndWhile
\EndProcedure

\hspace*{\fill}

\Procedure{Modulus}{}
    \State $\text{shift}_{1st} \gets 64 \div len_Y \ast len_Y$
    \State $\text{shift}_{2ed} \gets ((len_Y - 1) \mod len_{look\_up}) + 1$
    
    \State $\text{idx\_shift}_{1st} \gets len_Y - \text{shift}_{2st}$
    \State $\text{idx\_shift}_{2ed} \gets len_Y - len_{look\_up}$
    
    \State $\text{MAX\_2ED\_SHIFT} \gets \lceil len_Y \mod  len_{look\_up} \rceil$
    \State $\text{SHARED\_SIZE} == 2^{len_{look\_up}}$

    \hspace*{\fill}

    \State $i_{\text{init}} \gets (\text{blockIdx.x} \times \text{blockDim.x} + \text{threadIdx.x}) \times P$

    \State \textbf{shared} $\text{uint64\_t}$ \text{shared\_table[SHARED\_SIZE]}
    
    \If{$\text{threadIdx.x} < \text{table\_size}$}
        \State \text{shared\_table[threadIdx.x]} $\gets$ \text{table[threadIdx.x]}
    \EndIf
    \State \textbf{sync threads}

    \hspace*{\fill}
    
    \For{$i \gets i_{\text{init}}$ \textbf{to} $i_{\text{init}} + P$ \textbf{and} $i < \text{size}$}
        \State $\text{numX} \gets X[i]$
        \State $\text{T} \gets \text{numX} \gg \text{shift}_{1st} $

        \For{$\text{shift} \gets \text{shift}_{1st} - len_Y$ \textbf{down to} $0$ \textbf{by} $len_Y$}
            \State $\text{next} \gets (\text{numX} \gg \text{shift}) \& \text{digits}$

            \State $\text{idx} \gets \text{T} \gg \text{idx\_shift}_{1st} $
            \State $\text{T} \gets \text{T} \ll \text{shift}_{2ed}$
            
            \If{$\text{idx} \neq 0$}
                \State $\text{T} \gets \text{T} + \text{shared\_table[T]}$
                \State $\text{Set\_higher\_bits\_0(T)}$
            \EndIf

            \For{$\text{j} \gets 1$ \textbf{up to} $\text{MAX\_2ED\_SHIFT}$ \textbf{by} $1$}        
                \State $\text{idx} \gets \text{T} \gg \text{idx\_shift}_{2ed}$

                \State $\text{T} \ll len_{look\_up}$
                \State $\text{T} \gets T \& \text{digits} + \text{shared\_table[idx]}$

                \State $\text{Set\_higher\_bits\_0(T)}$

            \EndFor

            \State $\text{T} \gets \text{T} + \text{next}$

            \State $\text{Set\_higher\_bits\_0(T)}$
        \EndFor
        
        \State $\text{result[i]} \gets (\text{T} \ge Y) \, ? \, (\text{T} - Y) \, : \, \text{T}$
    \EndFor
\EndProcedure
\end{algorithmic}
\end{algorithm}
\clearpage

%\subsection*{Appendix B: Performance for operators in BGV}

% \begin{sidewaystable}[htb]
\begin{table*}[!h]
\caption{Running time in $\mu$s and speed up times for all BGV operators}\label{bgv-operator}
% \begin{tabular*}{\textwidth}{@{\extracolsep{\fill}}llrrrrr}
\begin{tabular*}{\linewidth}{@{\extracolsep{\fill}}llrrrrr}
\toprule
                                   & Operator                  & SEAL(CPU) & \emph{CAT}(3090) & \textbf{Speed} & \emph{CAT}(4090) & \textbf{Speed} \\ \hline

                                   & encode\_batch             & 640     & 466           & \textbf{1x}    & 371            & \textbf{2x}    \\
                                   & encode\_unbatch           & 773     & 527           & \textbf{1x}    & 480            & \textbf{2x}    \\
                                   & encrypt                   & 98133     & 1432            & \textbf{50x}   & 1294            & \textbf{76x}    \\
   \multirow{6}{*}{ BGV} 
                                   & decrypt                   & 19376      & 762              & \textbf{25x}  & 519             & \textbf{37}    \\
                                   
   \multirow{7}{*}{ N=32768, L=16, Q=881}
                                   & add                       & 4053      & 10               & \textbf{405x}  & 6              & \textbf{676x}    \\
                                   & multiply                  & 8762      & 23              & \textbf{381x}  & 17              & \textbf{515x}   \\
                                   & multiply\_plain           & 15433      & 420               & \textbf{37x}  & 191               & \textbf{81x}  \\
                                   & square                    & 10865      & 6              & \textbf{1810x}  & 5              & \textbf{2173x}   \\
                                   & relinearize               & 193632    & 4979            & \textbf{39x}   & 3169            & \textbf{61x}    \\
                                   & rotate\_rows\_one\_step & 203200    & 4182            & \textbf{49x}   & 2981            & \textbf{68x}    \\
                                   & rotate\_rows\_random    & 872223    & 16847           & \textbf{52x}   & 11837           & \textbf{74x}    \\
                                   & rotate\_columns    & 196284    & 4018           & \textbf{49x}   & 2786           & \textbf{70x}    \\
                                   \bottomrule 

\end{tabular*}
% \end{sidewaystable}
\end{table*}
%\textbf{Appendix B: Performance for operators in BGV}
%\section*{Appendix B: Performance for operators in BGV}
